# Supplementary material for: Three-Dimensional Anderson Localization in Variable Scale Disorder
Source: arXiv:1307.7175 ancillary file (2013-07-26)
Supplement: Supplementary file 1 [file SM.pdf]

# Supplemental Material for "3D Anderson Localization in Variable Scale Disorder"

W. R. McGehee,[1] S. S. Kondov,[1] W. Xu,[1] J. J. Zirbel,[1,*] and B. DeMarco[1]

[1]*Department of Physics, University of Illinois at Urbana-Champaign, Urbana, Illinois 61801, USA*

(Dated: July 26, 2013)

## EXPERIMENTAL PARAMETERS

The harmonic frequencies of the dipole trap are $\omega_x = 2\pi \times (45 \pm 1)$ Hz and $\omega_y = \omega_z = 2\pi \times (95 \pm 1)$ Hz. At the focal plane of the lens, the speckle intensity has a Gaussian envelope with a 170 $\mu$m $1/e^2$ radius, which does not depend on the aperture of the focusing lens. The Rayleigh length of the speckle intensity envelope varies from 400–1200 $\mu$m as the diameter of the aperture is varied. The disorder strength $\Delta$ is calibrated to within 10% statistical uncertainty by measuring the dipole force from the speckle envelope. There is a systematic uncertainty in $\Delta$ related to measuring the speckle envelope that is less than 40%. The speckle potential does not support classically bound states at relevant energy scales [1].

## SPECKLE AUTOCORRELATION CHARACTERIZATION

The speckle autocorrelation lengths for different focusing lens aperture diameters were measured by imaging the 3D speckle intensity distribution. The speckle intensity near the focus was reconstructed in 3D using two-dimensional slices imaged with a microscope formed by an objective and CCD camera with a combined magnification of 66 nm/pixel, resolution of 0.2 $\mu$m, and depth-of-field of 0.4 $\mu$m. The microscope was mounted on a 3-axis translation stage adjustable in 0.5 $\mu$m steps, and scans include 45–75 images taken with 0.5–5 $\mu$m spacing. Sub-pixel jitter between frames was removed by measuring the phase correlation between adjacent frames in the reconstruction and re-aligning the images using the Fourier shift theorem. The measured intensity autocorrelation is shown in Fig. 1 for 4.7–15.1 mm aperture diameters.

The exact form of the autocorrelation is complicated by truncation of the Gaussian profile (with a 6.66 mm waist) of the speckle laser beam at the imaging pupil. The observed autocorrelation is consistent with predictions for focusing a truncated Gaussian beam [2]. For simplicity, we fit two-dimensional slices of the the central correlation feature to a two-dimensional Gaussian. The fitted $1/e^2$ radii along each direction and the geometric mean $\overline{\zeta}$ are shown in Fig. 2.

A fit of the data for $\overline{\zeta}$ in Fig. 2 to a decaying exponential function is used to interpolate between aperture diameters and determine $\overline{\zeta}$ for Fig. 4 in the main text. There is less than a 5% uncertainty in $\overline{\zeta}$ determined using this method.

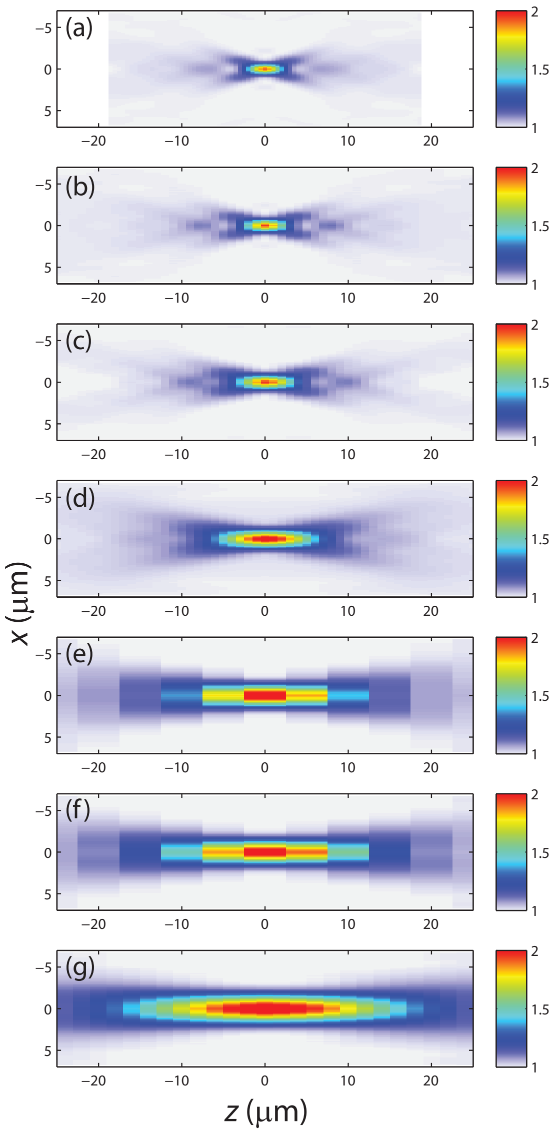


FIG. 1. The measured intensity autocorrelation is shown in false color for 15.1 (a), 11.2 (b), 9.9 (c), 7.9 (d), 6.3 (e), 5.7 (f), and 4.7 (g) mm aperture diameters. The color bars indicate the magnitude of the autocorrelation.

## STRETCHED EXPONENTIAL FIT

The data in Fig. 4 in the main text were obtained by fitting images to a stretched exponential. The variation of the stretch exponent $\beta$ with the correlation length $\overline{\zeta}$ is shown in Fig. 3. A decaying exponential is described by a fit with $\beta = 1$. The higher $\beta$ observed at larger $\overline{\zeta}$ indicates that the localized density profile is more peaked for longer speckle correlation lengths. The data in Fig. 2 in the main text were fit with fixed $\beta = 0.8$, which

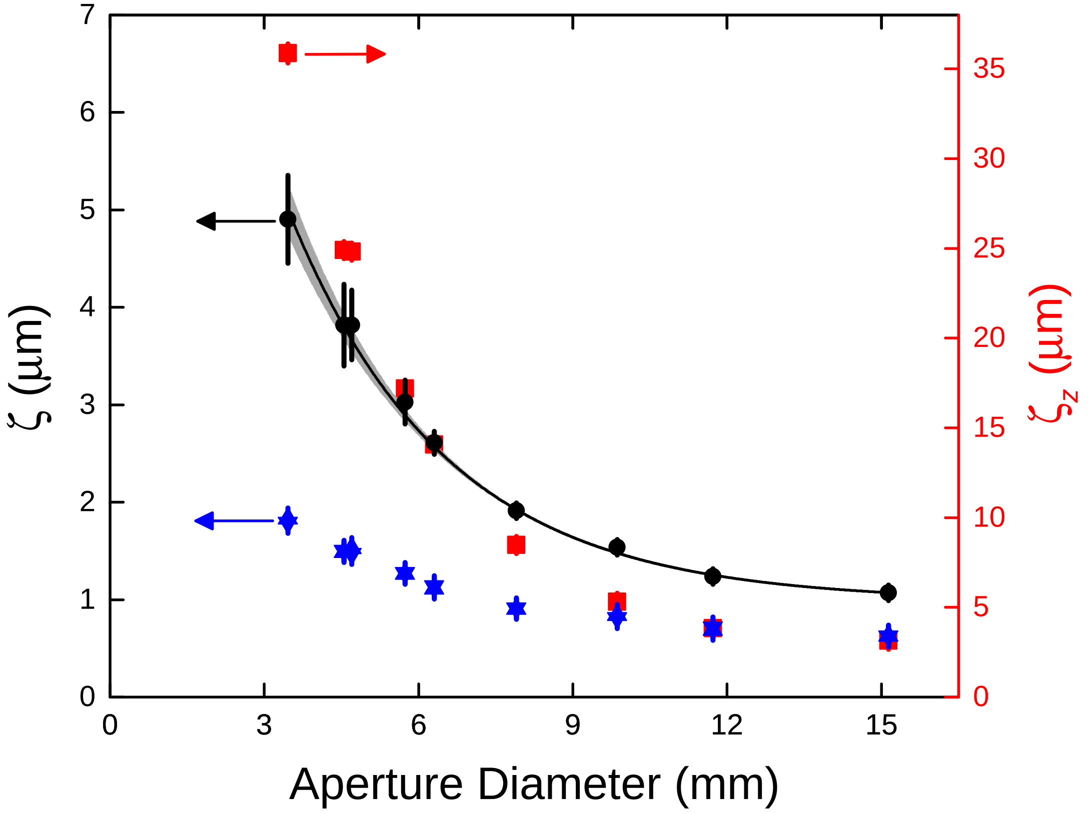


FIG. 2. Ex-situ characterization of the three-dimensional speckle autocorrelation function. The $x$ and $y$ directions are shown as blue upright and inverted triangles, and the $z$ direction is shown using red squares. The computed geometric mean $\bar{\zeta}$ is shown in black circles. The error bars for are determined by the uncertainty in the fit to the measured autocorrelation. The solid line is a fit to a decaying exponential used to interpolate between aperture diameters; the gray band shows the 68% confidence interval for this fit.

is the value for the unperturbed gas determined with $\beta$ as a free parameter.

---

* Now atAOSense, 767 N. Mary Ave., Sunnyvale, CA 94085


[1] S. Pilati, S. Giorgini, M. Modugno, and N. Prokof'ev, New J. Phys **12**, 073003 (2010).

[2] H. Urey, Appl. Opt. **43**, 620 (2004).

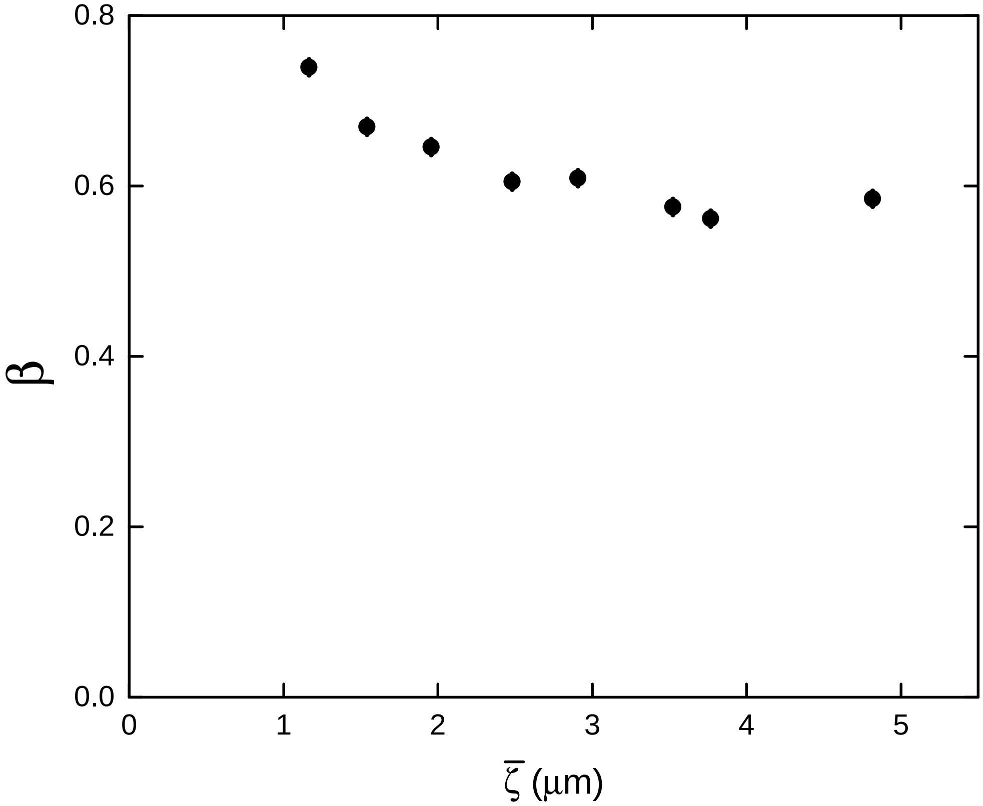


FIG. 3. Stretch exponent from the fits used to determine the RMS axial size of the gas $\sigma$ for the data in Fig. 4 in the main text. The error bars are the standard error in the mean for the 20 measurements that are averaged for each point.
